# Supplementary material for: RecDiff: Diffusion Model for Social Recommendation
Source: arXiv:2406.01629 source file (2024-06-01)
Supplement: Supplementary file 1 [file appendix.tex]

\section{Appendix}
